# Supplementary material for: Complete Verification via Multi-Neuron Relaxation Guided Branch-and-Bound
Source: arXiv:2205.00263 source file (2022-04-30)
Supplement: Supplementary file 1 [file appendix-labels-loader-1.tex]

% creates the file "appendix-labels.aux", with content from "appendix.aux"

\begin{filecontents}{appendix-labels.aux}

% STARTMARKER: start of auto-generated content
