# Supplementary material for: Complete Verification via Multi-Neuron Relaxation Guided Branch-and-Bound
Source: arXiv:2205.00263 source file (2022-04-30)
Supplement: Supplementary file 2 [file appendix-labels-loader-2.tex]

% ENDMARKER: end of auto-generated content
	
\end{filecontents}
